# Supplementary material for: On Parameters of Nonlinear Scalar Dynamics from Video: Invariants, Calibration, and Identifiability
Source: arXiv:2609.38877 source file (2026-09-30)
Supplement: Supplementary file 1 [file discussion_addendum.tex]

% Optional insertion at the end of appendix/operational_details.tex.
% This fragment adds no labels, headings with counters, or new assumptions.

\noindent\textbf{Compatible sets and realizable ambiguity.}
The general containment results give outer sets of parameters compatible
with the prescribed laws and covered trajectories. Constancy on such a set
is sufficient for identification, but variation alone does not show that a
fixed encoder class realizes the competing reports. For semilinear laws,
Proposition~\ref{prop:affine-realizability} supplies this converse when the
physical coordinate is representable and the encoder class is closed under
invertible affine output transformations. Only under these assumptions
does Corollary~\ref{cor:realizable-invariants} characterize identification by
constancy on the entire compatible set. This encoder-realizability result
is not asserted for the canonical sets merely because a raw--canonical
law equivalence holds. Likewise, failure of a sufficient coverage condition
or inability to audit a premise is not itself a parameter-nonidentifiability
proof. These cases must be distinguished from an explicit construction of
competing admissible reports.

\noindent\textbf{Structural identification and empirical accuracy.}
Exact representability is an assumption, and the constructed compatible
encoders need not be reached by the training objective. The deterministic
semilinear bounds transfer residual and approximation errors under the
stated regularity and physical-velocity conditioning; they are not
statistical confidence statements. The calibration criterion in
Proposition~\ref{prop:anchor-rank} also treats supplied anchor values as
exact and yields local uniqueness at regular points, not robustness to
measurement error or global uniqueness across branches. Empirical parameter
error, coordinate agreement, and sensitivity to initialization therefore
remain separate questions, as illustrated in
Appendices~\ref{app:exp-real-pendulum} and~\ref{app:exp-real-overhead}.
Repeated fits with shared observations or anchors describe variation under
that protocol, not uncertainty from independent physical measurements.
Propagating observation and anchor uncertainty into parameter guarantees
requires additional analysis beyond the current results.
